# Supplementary material for: ASTRA: Accurate and Scalable ANNS-based Training of Extreme Classifiers
Source: arXiv:2409.20156 source file (2024-09-30)
Supplement: Supplementary file 1 [file lfat_131k_appendix.tex]

\begin{table*}[]
\caption{Comparison of state-of-the-art and baseline XC methods.}
\vskip 0.1in

\begin{tabular}{@{}lllllll@{}}
\toprule
\multirow{2}{*}{Methods}            & \multicolumn{6}{c}{LF-AmazonTitles-131K}                                                \\ \cmidrule(l){2-7} 
                                    & P@1   & P@3   & \multicolumn{1}{l|}{P@5}   & PSP@1 & PSP@3 & \multicolumn{1}{l|}{PSP@5} \\ \midrule
\multicolumn{1}{|l|}{LEXUS}         & 45.83 & 30.4  & \multicolumn{1}{l|}{21.58} & 39.49 & 45.29 & \multicolumn{1}{l|}{50.28} \\
\multicolumn{1}{|l|}{Renee}         & 46.05 & 30.81 & \multicolumn{1}{l|}{22.04} & 39.08 & 45.12 & \multicolumn{1}{l|}{50.48} \\
\multicolumn{1}{|l|}{DEXA}          & 46.42 & 30.5  & \multicolumn{1}{l|}{21.59} & 39.11 & 44.69 & \multicolumn{1}{l|}{49.65} \\
\multicolumn{1}{|l|}{NGAME}         & 46.01 & 30.28 & \multicolumn{1}{l|}{21.47} & 38.81 & 44.4  & \multicolumn{1}{l|}{49.43} \\
\multicolumn{1}{|l|}{SiameseXML}    & 41.42 & 27.92 & \multicolumn{1}{l|}{21.21} & 35.8  & 40.96 & \multicolumn{1}{l|}{46.19} \\
\multicolumn{1}{|l|}{ECLARE}        & 40.74 & 27.54 & \multicolumn{1}{l|}{19.88} & 33.51 & 39.55 & \multicolumn{1}{l|}{44.7}  \\
\multicolumn{1}{|l|}{GalaXC}        & 39.17 & 26.85 & \multicolumn{1}{l|}{19.49} & 32.5  & 38.79 & \multicolumn{1}{l|}{43.95} \\
\multicolumn{1}{|l|}{DECAF}         & 38.4  & 25.84 & \multicolumn{1}{l|}{18.65} & 30.85 & 36.44 & \multicolumn{1}{l|}{41.42} \\
\multicolumn{1}{|l|}{Astec}         & 37.12 & 25.2  & \multicolumn{1}{l|}{18.24} & 29.22 & 34.64 & \multicolumn{1}{l|}{39.49} \\
\multicolumn{1}{|l|}{AttentionXML}  & 32.25 & 21.7  & \multicolumn{1}{l|}{15.61} & 23.97 & 28.6  & \multicolumn{1}{l|}{32.57} \\
\multicolumn{1}{|l|}{MACH}          & 33.49 & 22.71 & \multicolumn{1}{l|}{16.45} & 24.97 & 30.23 & \multicolumn{1}{l|}{34.72} \\
\multicolumn{1}{|l|}{X-Transformer} & 29.95 & 18.73 & \multicolumn{1}{l|}{13.07} & 21.72 & 24.42 & \multicolumn{1}{l|}{27.09} \\
\multicolumn{1}{|l|}{LightXML}      & 35.6  & 24.15 & \multicolumn{1}{l|}{17.45} & 25.67 & 31.66 & \multicolumn{1}{l|}{36.44} \\
\multicolumn{1}{|l}{BERTXML}        & 38.89 & 26.17 & 18.72                      & 30.1  & 36.81 & \multicolumn{1}{l|}{41.85} \\
\multicolumn{1}{|l}{ELIAS}          & 40.13 & 27.11 & 19.54                      & 31.05 & 37.57 & \multicolumn{1}{l|}{42.88} \\
\multicolumn{1}{|l}{AnneXML}        & 30.05 & 21.25 & 16.02                      & 19.23 & 26.09 & \multicolumn{1}{l|}{32.26} \\
\multicolumn{1}{|l}{DiSMEC}         & 35.14 & 23.88 & 17.24                      & 25.86 & 32.11 & \multicolumn{1}{l|}{36.97} \\
\multicolumn{1}{|l}{Parabel}        & 32.6  & 21.8  & 15.61                      & 23.27 & 28.21 & \multicolumn{1}{l|}{32.14} \\
\multicolumn{1}{|l}{XT}             & 31.41 & 21.39 & 15.48                      & 22.37 & 27.51 & \multicolumn{1}{l|}{31.64} \\
\multicolumn{1}{|l}{Slice}          & 30.43 & 20.5  & 14.84                      & 23.08 & 27.74 & \multicolumn{1}{l|}{31.89} \\
\multicolumn{1}{|l}{PfastreXML}     & 32.56 & 22.25 & 16.05                      & 26.81 & 30.61 & \multicolumn{1}{l|}{34.24} \\
\multicolumn{1}{|l}{Bonsai}         & 34.11 & 23.06 & 16.63                      & 24.75 & 30.35 & \multicolumn{1}{l|}{34.86} \\
\multicolumn{1}{|l}{XR-Transformer} & 38.1  & 25.57 & 18.32                      & 28.86 & 34.85 & \multicolumn{1}{l|}{39.59} \\ \bottomrule
\end{tabular}

\vskip -0.1in
\end{table*}
