# Supplementary material for: ASTRA: Accurate and Scalable ANNS-based Training of Extreme Classifiers
Source: arXiv:2409.20156 source file (2024-09-30)
Supplement: Supplementary file 2 [file lfa_131k_appendix.tex]

\begin{table*}[]
\caption{Comparison of state-of-the-art and baseline XC methods.}
\vskip 0.1in

\begin{tabular}{@{}lllllll@{}}
\toprule
\multirow{2}{*}{Methods}         & \multicolumn{6}{c}{LF-Amazon-131K}                                                      \\ \cmidrule(l){2-7} 
                                 & P@1   & P@3   & \multicolumn{1}{l|}{P@5}   & PSP@1 & PSP@3 & \multicolumn{1}{l|}{PSP@5} \\ \midrule
\multicolumn{1}{|l|}{LEXUS}      & 47.13 & 31.29 & \multicolumn{1}{l|}{22.35} &       &       & \multicolumn{1}{l|}{}      \\
\multicolumn{1}{|l|}{Renee}      & 48.05 & 32.33 & \multicolumn{1}{l|}{23.26} &       &       & \multicolumn{1}{l|}{}      \\
\multicolumn{1}{|l|}{DEXA}       & 47.16 & 31.45 & \multicolumn{1}{l|}{22.42} & 38.7  & 45.43 & \multicolumn{1}{l|}{50.97} \\
\multicolumn{1}{|l|}{NGAME}      & 46.53 & 30.89 & \multicolumn{1}{l|}{22.02} & 38.53 & 44.95 & \multicolumn{1}{l|}{50.45} \\
\multicolumn{1}{|l|}{SiameseXML} & 44.81 & 30.19 & \multicolumn{1}{l|}{21.94} & 37.56 & 43.69 & \multicolumn{1}{l|}{49.75} \\
\multicolumn{1}{|l|}{ECLARE}     & 43.56 & 29.65 & \multicolumn{1}{l|}{21.57} & 34.98 & 42.38 & \multicolumn{1}{l|}{48.53} \\
\multicolumn{1}{|l|}{GalaXC}     & 41.46 & 28.04 & \multicolumn{1}{l|}{20.25} & 35.1  & 41.18 & \multicolumn{1}{l|}{46.38} \\
\multicolumn{1}{|l|}{DECAF}      & 42.94 & 28.79 & \multicolumn{1}{l|}{21}    & 34.52 & 41.14 & \multicolumn{1}{l|}{47.33} \\
\multicolumn{1}{|l|}{Astec}      & 42.22 & 28.62 & \multicolumn{1}{l|}{20.85} & 32.95 & 39.42 & \multicolumn{1}{l|}{45.3}  \\ \midrule
AttentionXML                     & 42.9  & 28.96 & 20.97                      & 32.92 & 39.51 & 45.24                      \\
MACH                             & 34.52 & 23.39 & 17                         & 25.27 & 30.71 & 35.42                      \\
LightXML                         & 41.49 & 28.32 & 20.75                      & 30.27 & 37.71 & 44.1                       \\
BERTXML                          & 42.59 & 28.39 & 20.27                      & 33.55 & 40.83 & 46.4                       \\
AnneXML                          & 35.73 & 25.46 & 19.41                      & 23.56 & 31.97 & 39.95                      \\
DiSMEC                           & 41.68 & 28.32 & 20.58                      & 31.61 & 38.96 & 45.07                      \\
Parabel                          & 39.57 & 26.64 & 19.26                      & 28.99 & 35.36 & 40.69                      \\
XT                               & 34.31 & 23.27 & 16.99                      & 24.35 & 29.81 & 34.7                       \\
Slice                            & 32.07 & 22.21 & 16.52                      & 23.14 & 29.08 & 34.63                      \\
PfastreXML                       & 35.83 & 24.35 & 17.6                       & 28.99 & 33.24 & 37.4                       \\
Bonsai                           & 40.23 & 27.29 & 19.87                      & 29.6  & 36.52 & 42.39                      \\
XR-Transformer                   & 45.61 & 30.85 & 22.32                      & 34.93 & 42.83 & 49.24                      \\ \bottomrule
\end{tabular}
\vskip -0.1in
\end{table*}
