# Supplementary material for: ASTRA: Accurate and Scalable ANNS-based Training of Extreme Classifiers
Source: arXiv:2409.20156 source file (2024-09-30)
Supplement: Supplementary file 3 [file lfat13M_appendix.tex]

\begin{table*}[]
\caption{Comparison of state-of-the-art and baseline XC methods.}
\vskip 0.1in

\begin{tabular}{@{}lllllll@{}}
\toprule
\multirow{2}{*}{Methods}         & \multicolumn{6}{c}{LF-AmazonTitles-1.3M}                                                \\ \cmidrule(l){2-7} 
                                 & P@1   & P@3   & \multicolumn{1}{l|}{P@5}   & PSP@1 & PSP@3 & \multicolumn{1}{l|}{PSP@5} \\ \midrule
\multicolumn{1}{|l|}{LEXUS}      & 55.50 & 48.82 & \multicolumn{1}{l|}{44.15} & 30.16 & 34.39 & \multicolumn{1}{l|}{36.82} \\
\multicolumn{1}{|l|}{Renee}      & 56.04 & 49.91 & \multicolumn{1}{l|}{45.32} & 28.54 & 33.38 & \multicolumn{1}{l|}{36.14} \\
\multicolumn{1}{|l|}{DEXA}       & 56.63 & 49.05 & \multicolumn{1}{l|}{43.9}  & 29.12 & 32.69 & \multicolumn{1}{l|}{34.86} \\
\multicolumn{1}{|l|}{NGAME}      & 56.75 & 49.19 & \multicolumn{1}{l|}{44.09} & 29.18 & 33.01 & \multicolumn{1}{l|}{35.36} \\
\multicolumn{1}{|l|}{SiameseXML} & 49.02 & 42.72 & \multicolumn{1}{l|}{38.52} & 27.12 & 30.43 & \multicolumn{1}{l|}{32.52} \\
\multicolumn{1}{|l|}{ECLARE}     & 50.14 & 44.09 & \multicolumn{1}{l|}{40}    & 23.43 & 27.9  & \multicolumn{1}{l|}{30.56} \\
\multicolumn{1}{|l|}{GalaXC}     & 49.81 & 44.23 & \multicolumn{1}{l|}{40.12} & 25.22 & 29.12 & \multicolumn{1}{l|}{31.44} \\
\multicolumn{1}{|l|}{DECAF}      & 50.67 & 44.49 & \multicolumn{1}{l|}{40.35} & 22.07 & 26.54 & \multicolumn{1}{l|}{29.3}  \\
\multicolumn{1}{|l|}{Astec}      & 48.82 & 42.62 & \multicolumn{1}{l|}{38.44} & 21.47 & 25.41 & \multicolumn{1}{l|}{27.86} \\ \midrule
AttentionXML                     & 45.04 & 39.71 & 36.25                      & 15.97 & 19.9  & 22.54                      \\
MACH                             & 35.68 & 31.22 & 28.35                      & 9.32  & 11.65 & 13.26                      \\
X-Transformer                    & -     & -     & -                          & -     & -     & -                          \\
LightXML                         & -     & -     & -                          & -     & -     & -                          \\
AnneXML                          & 47.79 & 41.65 & 36.91                      & 15.42 & 19.67 & 21.91                      \\
DiSMEC                           & -     & -     & -                          & -     & -     & -                          \\
Parabel                          & 46.79 & 41.36 & 37.65                      & 16.94 & 21.31 & 24.13                      \\
XT                               & 40.6  & 35.74 & 32.01                      & 13.67 & 17.11 & 19.06                      \\
Slice                            & 34.8  & 30.58 & 27.71                      & 13.96 & 17.08 & 19.14                      \\
PfastreXML                       & 37.08 & 33.77 & 31.43                      & 28.71 & 30.98 & 32.51                      \\
Bonsai                           & 47.87 & 42.19 & 38.34                      & 18.48 & 23.06 & 25.95                      \\
XR-Transformer                   & 50.14 & 44.07 & 39.98                      & 20.06 & 24.85 & 27.79                      \\ \bottomrule
\end{tabular}

\vskip -0.1in
\end{table*}
