# Supplementary material for: ASTRA: Accurate and Scalable ANNS-based Training of Extreme Classifiers
Source: arXiv:2409.20156 source file (2024-09-30)
Supplement: Supplementary file 4 [file wiki_appendix.tex]

\begin{table*}[]
\caption{Comparison of state-of-the-art and baseline XC methods.}
\vskip 0.1in

\begin{tabular}{@{}lllllll@{}}
\toprule
\multirow{2}{*}{Methods}         & \multicolumn{6}{c}{LF-Wikipedia-500K}                                                   \\ \cmidrule(l){2-7} 
                                 & P@1   & P@3   & \multicolumn{1}{l|}{P@5}   & PSP@1 & PSP@3 & \multicolumn{1}{l|}{PSP@5} \\ \midrule
\multicolumn{1}{|l|}{LEXUS}      & 84.65 & 66.09 & \multicolumn{1}{l|}{51.50} &       &       & \multicolumn{1}{l|}{}      \\
\multicolumn{1}{|l|}{Renee}      & 84.95 & 66.25 & \multicolumn{1}{l|}{51.68} &       &       & \multicolumn{1}{l|}{}      \\
\multicolumn{1}{|l|}{DEXA}       & 84.92 & 65.5  & \multicolumn{1}{l|}{50.51} & 42.59 & 53.93 & \multicolumn{1}{l|}{58.33} \\
\multicolumn{1}{|l|}{NGAME}      & 84.01 & 64.69 & \multicolumn{1}{l|}{49.97} & 41.25 & 52.57 & \multicolumn{1}{l|}{57.04} \\
\multicolumn{1}{|l|}{SiameseXML} & 67.26 & 44.82 & \multicolumn{1}{l|}{33.73} & 33.95 & 35.46 & \multicolumn{1}{l|}{37.07} \\
\multicolumn{1}{|l|}{ECLARE}     & 68.04 & 46.44 & \multicolumn{1}{l|}{35.74} & 31.02 & 35.39 & \multicolumn{1}{l|}{38.29} \\
\multicolumn{1}{|l|}{GalaXC}     & 55.26 & 35.07 & \multicolumn{1}{l|}{26.13} & 31.82 & 31.26 & \multicolumn{1}{l|}{32.47} \\
\multicolumn{1}{|l|}{DECAF}      & 73.96 & 54.17 & \multicolumn{1}{l|}{42.43} & 32.13 & 40.13 & \multicolumn{1}{l|}{44.59} \\
\multicolumn{1}{|l|}{Astec}      & 73.02 & 52.02 & \multicolumn{1}{l|}{40.53} & 30.69 & 36.48 & \multicolumn{1}{l|}{40.38} \\ \midrule
AttentionXML                     & 82.73 & 63.75 & 50.41                      & 34    & 44.32 & 50.15                      \\
MACH                             & 52.78 & 32.39 & 23.75                      & 17.65 & 18.06 & 18.66                      \\
X-Transformer                    & 76.95 & 58.42 & 46.14                      & -     & -     & -                          \\
LightXML                         & 81.59 & 61.78 & 47.64                      & 31.99 & 42    & 46.53                      \\
AnneXML                          & 64.64 & 43.2  & 32.77                      & 26.88 & 30.24 & 32.79                      \\
DiSMEC                           & 70.2  & 50.6  & 39.7                       & 31.2  & 33.4  & 37                         \\
Parabel                          & 68.7  & 49.57 & 38.64                      & 26.88 & 31.96 & 35.26                      \\
XT                               & 64.48 & 45.84 & 35.46                      & -     & -     & -                          \\
PfastreXML                       & 59.5  & 40.2  & 30.7                       & 29.2  & 27.6  & 27.7                       \\
Bonsai                           & 69.2  & 49.8  & 38.8                       & 27.46 & 32.25 & 35.48                      \\
XR-Transformer                   & 81.62 & 61.38 & 47.85                      & 33.58 & 42.97 & 47.81                      \\
XR-Transformer                   &       &       &                            &       &       &                            \\ \bottomrule
\end{tabular}
\vskip -0.1in
\end{table*}
